# Supplementary material for: Structural disorder by octahedral tilting in inorganic halide perovskites: New insight with Bayesian optimization
Source: arXiv:2303.08426 source file (2023-03-15)
Supplement: Supplementary file 1 [file supporting_information.pdf]

# Supporting Information *for* Structural Disorder by Octahedral Tilting in Inorganic Halide Perovskites: New Insight with Bayesian Optimization

*Jingrui Li*[*1], *Fang Pan* [1], *Guo-Xu Zhang* [2], *Zenghui Liu* [1], *Hua Dong* [3], *Dawei Wang* [4], *Zhuangde Jiang* [5], *Wei Ren*[1], *Zuo-Guang Ye* [6], *Milica Todorović*[**7], *Patrick Rinke* [8]

[1] Electronic Materials Research Laboratory, Key Laboratory of the Ministry of Education and International Center for Dielectric Research, School of Electronic Science and Engineering & International Joint Laboratory for Micro/Nano Manufacturing and Measurement Technology, Xi'an Jiaotong University, Xi'an 710049, China

[2] MIIT Key Laboratory of Critical Materials Technology for New Energy Conversion and Storage, School of Chemistry and Chemical Engineering, Harbin Institute of Technology, Harbin 150001, China

[3] Key Laboratory for Physical Electronics and Devices of the Ministry of Education and Shaanxi Key Lab of Information Photonic Technique, School of Electronic Science and Engineering, Xi'an Jiaotong University, Xi'an 710049, China

[4] School of Microelectronics and Key Lab of Micro-Nano Electronics and System Integration of Xi'an City, Xi'an Jiaotong University, Xi'an 710049, China

[5] State Key Laboratory for Manufacturing Systems Engineering & International Joint Laboratory for Micro/Nano Manufacturing and Measurement Technology, Xi'an Jiaotong University, Xi'an 710049, China

[6] Department of Chemistry and 4D LABS, Simon Fraser University, Burnaby, British Columbia V5A 1S6, Canada

[7] Department of Mechanical and Materials Engineering, University of Turku, FI-20014 Turku, Finland

[8] Department of Applied Physics, Aalto University, P.O.Box 11100, FI-00076 AALTO, Finland

* jingrui.li@xjtu.edu.cn

** milica.todorovic@utu.fi

## S1 DFT full relaxation results for several tilting patterns

**Table S1** shows the DFT full-relaxation results of $CsPbI_3$ and $CsPbBr_3$ initialized at several tilting patterns. In each listed data, the structure stays at its initial symmetry after relaxation. Not all results of Glazer's tiltings (e.g., in the Woodward's convention) are listed, since some of them fall into nearly identical relaxed structures (with only numerical difference in total energy, lattice constants, and atomic positions).

Table S1: Total energies (in meV per perovskite unit vs. $a^0a^0a^0$) of $CsPbX_3$ structures at different symmetries calculated with DFT full relaxation.

| Tilting | BOSS search space | Space group | $CsPbI_3$ | $CsPbBr_3$ |
|---|---|---|---|---|
| $a^+a^+a^+$ | ppp | $Im\bar{3}$ | −64.6 | −50.9 |
| $a^+a^+c^0$ | ppp, ppm | $I4/mmm$ | −74.2 | −57.3 |
| $a^+b^0b^0$ | ppp, ppm, pmm | $P4/mbm$ | −91.5 | −71.4 |
| $a^+b^-c^0$ | ppm, pmm | $Cmcm$ | −104.1 | −78.3 |
| $a^+b^-b^-$ | pmm | $Pnma$ | −132.6 | −97.3 |
| $a^-b^0b^0$ | ppm, pmm, mmm | $I4/mcm$ | −91.9 | −72.4 |
| $a^-a^-c^0$ | pmm, mmm | $Imma$ | −86.6 | −68.3 |
| $a^-b^-c^0$ | pmm, mmm | $C2/m$ | −93.7 | −73.2 |
| $a^-a^-a^-$ | mmm | $R\bar{3}c$ | −75.3 | −69.6 |

## S2 Symmetry-equivalent images of tilted structures in tilting-pattern-specific spaces and total space

For each tilting pattern, **Table S2** lists the numbers of symmetry-equivalent points in the configuration spaces. We should notice that for a given tilting pattern, the number is different for different configuration space. Using $a^+b^0b^0$ as an example, denoting the single in-phase tilting angle by $\theta$, the symmetry images are $(\theta_a, 0, 0)$, $(-\theta_a, 0, 0)$, $(0, \theta_a, 0)$, $(0, -\theta_a, 0)$, $(0, 0, \theta_a)$, and $(0, 0, -\theta_a)$ in ppp; $(\theta_a, 0, 0)$, $(-\theta_a, 0, 0)$, $(0, \theta_a, 0)$, and $(0, -\theta_a, 0)$ in ppm; $(\theta_a, 0, 0)$ and $(-\theta_a, 0, 0)$ in pmm; $(\theta_a, 0, 0)$, $(0, \theta_a, 0)$, and $(0, 0, \theta_a)$ in the total space.

Table S2: Number of symmetry-equivalent data points of each non-equivalent Glazer tilting within different search spaces and the total configuration space.

| Tilting | ppp | ppm | pmm | mmm | total space |
|---|---|---|---|---|---|
| $a^0a^0a^0$ | 1 | 1 | 1 | 1 | 1 |
| $a^+b^0b^0$ | 6 | 4 | 2 | | 3 |
| $a^-b^0b^0$ | | 2 | 4 | 6 | 3 |
| $a^+a^+c^0$ | 12 | 4 | | | 3 |
| $a^+b^+c^0$ | 24 | 8 | | | 6 |
| $a^+b^-c^0$ | | 8 | 8 | | 6 |
| $a^-a^-c^0$ | | | 4 | 12 | 3 |
| $a^-b^-c^0$ | | | 8 | 24 | 6 |
| $a^+a^+a^+$ | 8 | | | | 1 |
| $a^+a^+c^+$ | 24 | | | | 3 |
| $a^+b^+c^+$ | 48 | | | | 6 |
| $a^+a^+c^-$ | | 8 | | | 3 |
| $a^+b^+c^-$ | | 16 | | | 6 |
| $a^+b^-b^-$ | | | 8 | | 3 |
| $a^+b^-c^-$ | | | 16 | | 6 |
| $a^-a^-a^-$ | | | | 8 | 1 |
| $a^-a^-c^-$ | | | | 24 | 3 |
| $a^-b^-c^-$ | | | | 48 | 6 |

## S3 Further 2D cross-sections of 3D PESs

In the main text we have shown several representative 2D cross-sections of PESs in Figure 1. They mainly focus on pmm where the global minimum locates, together with three border planes successively separating ppp, ppm, pmm, and mmm. Here we put further 2D cross-sections that contain the minima (white dots) within ppp, ppm, and mmm in **Figure S1**.

From top to bottom of Figure S1:

1. $a^+b^+$ cross-section that contains the minimum of ppp ($c^+ = c^+_\mathrm{m}$): the lowest-energy locates at $a = b = 0°$, and is strongly bound around it.
2. $a^+c^-$ cross-section that contains the minimum of ppm ($b^+ = b^+_\mathrm{m}$): with one in-phase tilt ($b^+$) at the minimum, the other ($a^+$) is strongly limited at $a = 0$, while a small-angle out-of-phase tilt ($c^-$) stabilizes the structure. The system can fluctuate between $a^0b^+_\mathrm{m}c^-$ and $a^0b^+_\mathrm{m}(-c)^-$.
3. $a^+b^+$ cross-section that contains the minimum of ppm ($c^- = c^-_\mathrm{m}$): for $CsPbI_3$ , the system would be relatively constrained at each minimum but not easy to travel to its neighbor (e.g., $a^+b^0 \to a^0b^+$. The barrier for such a mode-switch for $CsPbBr_3$ is lower, leading to stronger structural disorder even at room temperature.
4. Two cross-sections containing the minimum of mmm, with $a^-_\mathrm{m}$ indicating the larger deviation from 0° at the minimum while $b^-_\mathrm{m}$ the smaller: the mode-switch between out-of-phase tilts is much easier than between in-phase tilts.

Overall, $CsPbBr_3$ displays more pronounced structures in these 2D PESs than $CsPbI_3$ . This corresponds to the more significant structural disorder in this perovskite.

(a) $CsPbI_3$ (b) $CsPbBr_3$

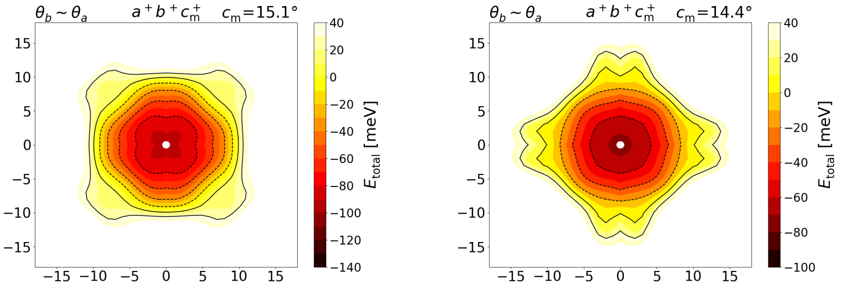


carried forward

continued

(a) $CsPbI_3$ (b) $CsPbBr_3$

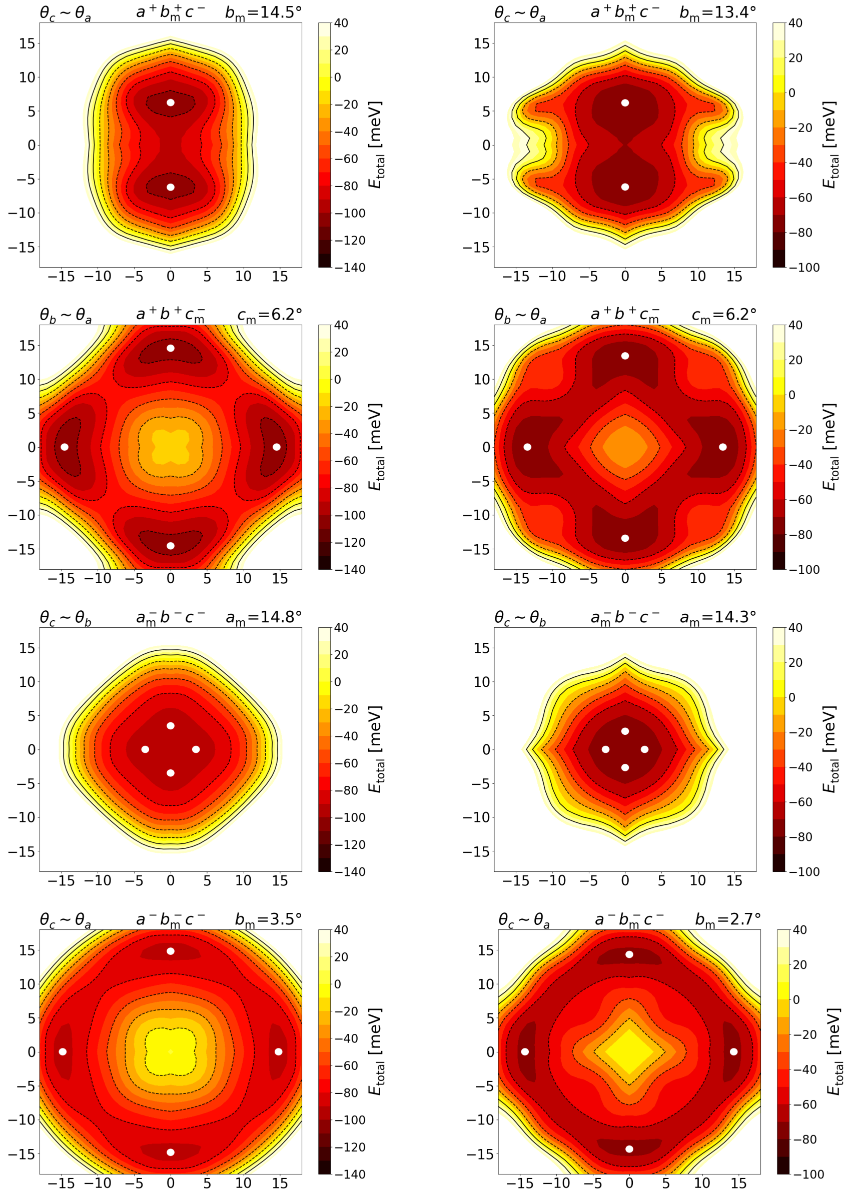


Figure S1: Some 2D cross-sections of 3D PESs of (a) $CsPbI_3$ and (b) $CsPbBr_3$ . From top to bottom: $a^+b^+$ with $c^{(+)}$ at its value at the minimum of ppp, $a^+c^-$ consisting of the minimum of ppm, $a^+b^+$ consisting of the minimum of ppm, and two planes containing the minimum of mmm with larger $(a_\mathrm{m}^-)$ and smaller $(b_\mathrm{m})$ coordinates.

## S4 MEPs linking global minima calculated by NEB method based on BOSS PESs

Table S3 lists the structure and barrier parameters of MEPs evaluated using NEB. In addition to the MEPs already discussed in the main text (labeled by "3D pmm" in Table S3), we have also performed NEB evaluation of MEPs within a series of 2D PES cross-sections in a way similar to Ref. [1]. For the $a^+b^-b^-$ cross-section (Figure 2a,c in the main text) in which the tilting angles of both out-of-phase tilts in pmm are forced to be identical, the barriers of MEPs $a^+b^-b^- \rightarrow a^+b^0b^0 \rightarrow a^+(-b)^-(-b)^-$ are clearly higher than the lowest barriers found in the 3D approach. In fact, 3D-NEB does not result in this pathway, but rather an "indirect" MEP $a^+b^-b^- \rightarrow a^+b^-c^0 \rightarrow a^+b^-(-b)^- \rightarrow a^+b^0(-c)^- \rightarrow a^+(-b)^-(-b)^-$ (i.e., two consecutive lowest-barrier MEPs). Transition-state structures $a^+b^-c^0$ are found in both $a^+_{\mathrm{m}}b^-c^-$ and $a^+b^-_{\mathrm{m}}c^-$ cross-sections. Their energies are slightly but noticeably higher than the 3D-MEP barriers (especially for $CsPbI_3$) because the tilting angle of the third mode is fixed in 2D approaches. In addition, MEPs that connect global minima in the other tilting-pattern-specific spaces are also provided, accordingly labeled by 3D ppm, 3D mmm, 3D ppp. These data help estimate whether direction reversal or tilting-mode exchange is easy to occur for different tilting patterns. For example, the barriers for the transfer of one in-phase tilt from one lattice vector to another is as high as $\sim$ 20 meV, while the barrier of the path to commute two out-of-phase tilts is much lower ($\sim$ 10 meV).

Table S3: Barriers and transition-state tilting patterns of MEPs that link global minima in different configuration spaces. The tilting angles of all starting structures are positive (except zero tilts). The superscript of tilting angles in transition-state structures denote the in-phase or out-of-phase tilt, while the negative sign within the parentheses indicates tilting in an opposite direction.

| Configuration space | Starting and ending structures | Transition-state structure $\theta_a$ [°] | $\theta_b$ [°] | $\theta_c$ [°] | Barrier [meV] |
|---|---|---|---|---|---|
| $CsPbI_3$ | | | | | |
| 3D pmm | $a^+b^-b^- \to a^+(-b)^-(-b)^-$ | $(14.1)^+$ | $(6.8)^-$ | 0 | 25.7 |
| | | $(14.1)^+$ | 0 | $(-6.8)^-$ | |
| | $a^+b^-b^- \to (-a)^+b^-b^-$ | 0 | $(14.6)^-$ | $(3.1)^-$ | 35.9 |
| | $a^+b^-b^- \to a^+b^-(-b)^-$ | $(14.1)^+$ | $(6.8)^-$ | 0 | 25.7 |
| 2D $a^+b^-b^-$ | $a^+b^-b^- \to a^+(-b)^-(-b)^-$ | $(15.1)^+$ | 0 | 0 | 37.4 |
| | $a^+b^-b^- \to (-a)^+b^-b^-$ | 0 | $(10.3)^-$ | $(10.3)^-$ | 44.5 |
| 2D $a^+_{\mathrm{m}}b^-c^-$ | $a^+b^-b^- \to a^+b^-(-b)^-$ | $(12.2)^+$ | $(8.1)^-$ | 0 | 29.2 |
| 2D $a^+b^-_{\mathrm{m}}c^-$ | $a^+b^-b^- \to a^+b^-(-b)^-$ | $(12.8)^+$ | $(9.1)^-$ | 0 | 29.5 |
| | $a^+b^-b^- \to (-a)^+b^-b^-$ | 0 | $(9.1)^-$ | $(11.8)^-$ | 43.8 |
| 3D ppm | $a^+b^-c^0 \to a^+(-b)^-c^0$ | $(15.0)^+$ | 0 | 0 | 11.9 |
| 3D mmm | $a^-b^-c^0 \to b^-a^-c^0$ | $(10.2)^-$ | $(10.2)^-$ | 0 | 8.7 |
| 3D ppp | $a^+b^0b^0 \to a^0b^+a^0$ | $(11.1)^+$ | $(5.7)^+$ | $(2.4)^+$ | 19.3 |
| $CsPbBr_3$ | | | | | |
| 3D pmm | $a^+b^-b^- \to a^+(-b)^-(-b)^-$ | $(13.2)^+$ | $(7.0)^-$ | 0 | 16.4 |
| | | $(13.2)^+$ | 0 | $(-7.0)^-$ | |
| | $a^+b^-b^- \to (-a)^+b^-b^-$ | 0 | $(9.4)^-$ | $(9.4)^-$ | 23.1 |
| | $a^+b^-b^- \to a^+b^-(-b)^-$ | $(13.2)^+$ | $(7.0)^-$ | 0 | 16.4 |
| 2D $a^+b^-b^-$ | $a^+b^-b^- \to a^+(-b)^-(-b)^-$ | $(14.4)^+$ | 0 | 0 | 22.4 |
| | $a^+b^-b^- \to (-a)^+b^-b^-$ | 0 | $(9.5)^-$ | $(9.5)^-$ | 24.6 |
| 2D $a^+_{\mathrm{m}}b^-c^-$ | $a^+b^-b^- \to a^+b^-(-b)^-$ | $(11.1)^+$ | $(8.6)^-$ | 0 | 18.7 |
| 2D $a^+b^-_{\mathrm{m}}c^-$ | $a^+b^-b^- \to a^+b^-(-b)^-$ | $(12.1)^+$ | $(8.3)^-$ | 0 | 17.8 |
| | $a^+b^-b^- \to (-a)^+b^-b^-$ | 0 | $(8.3)^-$ | $(10.5)^-$ | 24.9 |
| 3D ppm | $a^+b^-c^0 \to a^+(-b)^-c^0$ | $(14.7)^+$ | 0 | 0 | 5.5 |
| 3D mmm | $a^-b^-c^0 \to b^-a^-c^0$ | $(10.8)^-$ | $(8.1)^-$ | 0 | 3.4 |
| 3D ppp | $a^+b^0b^0 \to a^0b^+a^0$ | $(5.1)^+$ | $(4.7)^+$ | $(8.8)^+$ | 19.5 |

# S5 Further 2D cross-sections of configuration space distribution at different temperatures

**Figure S2**a provides a complete profile of how $CsPbI_3$ is distributed over the phase space (with 2D cross-sections $a^+b^-b^-$ and $c = 0$), at temperatures ranging from 450 to 800 K. Some figures are already given in the main text. We included them here for an systematic view (see main text for 650 K). With increasing temperature, relative population of the system at regions away from the global minima.

Figure S2b supplements the high-temperature (500 K) profile for $CsPbBr_3$. Mode-switch is very prevalent at this temperature, giving rise to a high structural disorder.

(a) $CsPbI_3$

$a^+b^-b^-$ 450 K

$a^{\pm}b^{\pm}c^0$ 300 K

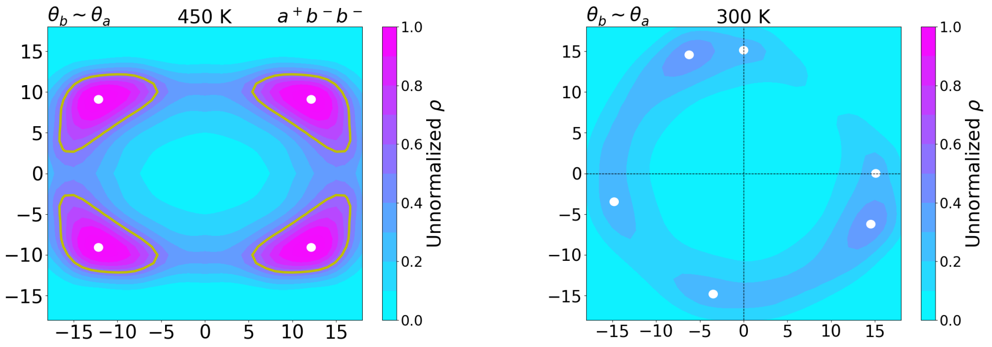


550 K

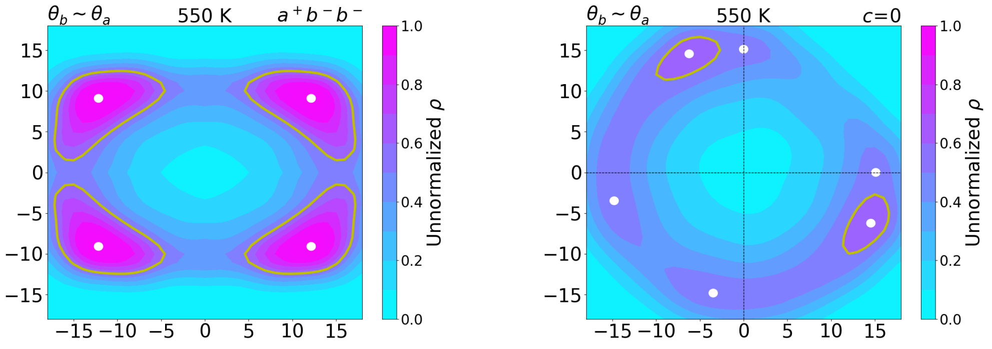


carried forward

continued

(a) $CsPbI_3$

$a^+b^-b^-$ $\qquad$ $a^\pm b^\pm c^0$

700 K

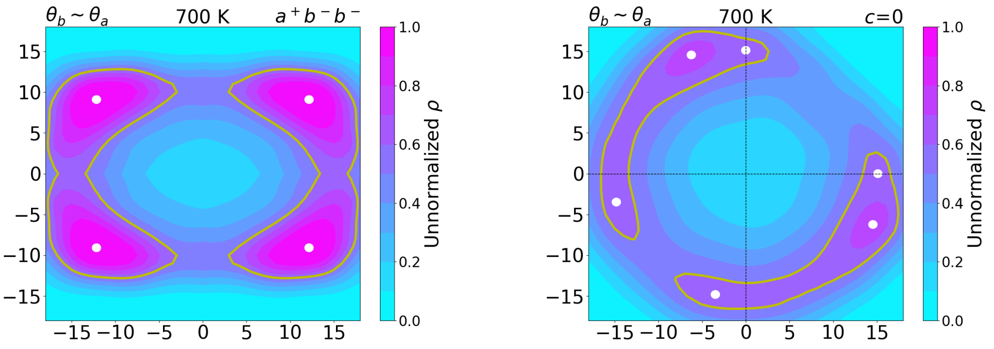


800 K

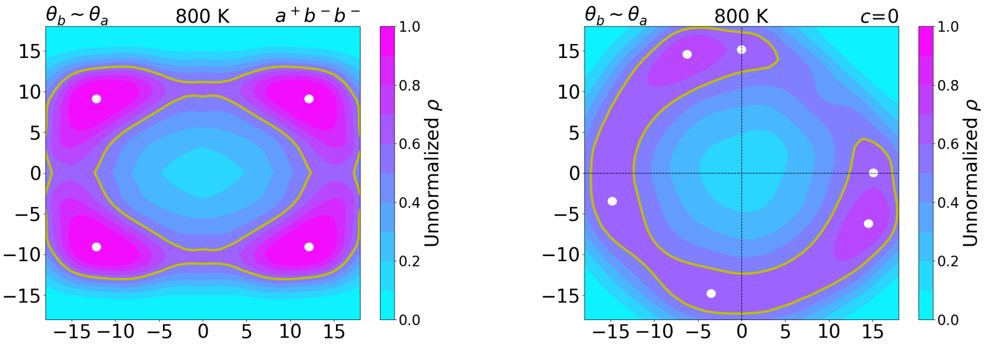


(b) $CsPbBr_3$

$a^+b^-b^-$ $\qquad$ $a^\pm b^\pm c^0$

500 K

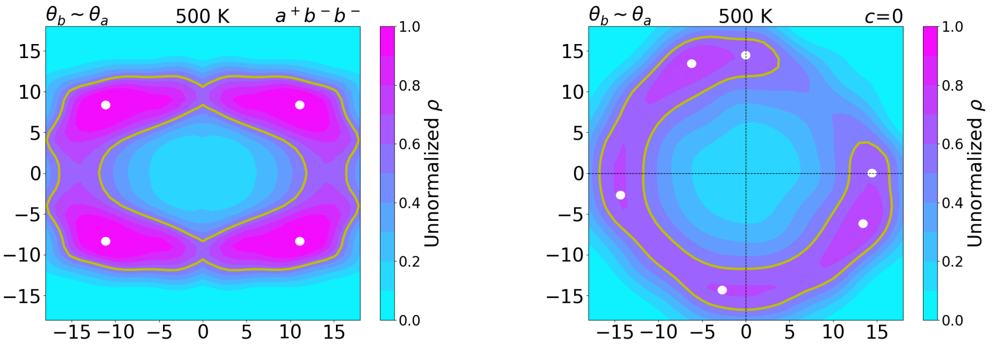


Figure S2: (a) 2D cross-sections ($a^+b^-b^-$ and $a^\pm b^\pm c^0$) of unnormalized distribution probability of $CsPbI_3$ at 450, 550, 700, and 800 K. (b) Tilting-angle distribution of $CsPbBr_3$ at 500 K.

## S6 A simplified approach to the surrogate model of PBEsol0+SOC band gaps

The underestimation of band gaps by generalized-gradient-approximation functionals (such as PBEsol used in this work) can be largely compensated by the omission of spin-orbit coupling (SOC) [2–4], higher-level first-principles calculations such as employing hybrid density functionals are nevertheless desirable for better accuracy. As a simpler alternative to the approach presented in the main text, we also made use of the relationship that the calculated band gap linearly depends on the proportion ($\alpha$) of Hartree-Fock (HF) exchange in the hybrid functional

$$E_{\mathrm{gap}}(\mathrm{PBEsol0{+}SOC}) = E_{\mathrm{gap}}(\mathrm{PBEsol}) + \alpha\Delta_{\mathrm{HF}} - \Delta_{\mathrm{SOC}}\,, \tag{1}$$

where $E_{\mathrm{gap}}$ is the band gap calculated by the method in the parentheses, $\alpha\Delta_{\mathrm{HF}}$ the correction (gap-opening) due to the HF exchange, and $\Delta_{\mathrm{SOC}}$ the Rashba-Dresselhaus band-gap reduction due to SOC. We performed PBEsol0 (with the default $\alpha = 0.25$) calculations at several PBEsol-optimized structures of different symmetries. **Figure S3** show that $\alpha\Delta_{\mathrm{HF}}$ stays quite constant for both compounds across all samples. $\Delta_{\mathrm{SOC}}$ fluctuates at different symmetries roughly between $\sim 0.6$ and $\sim 0.9$ eV. The studied materials exhibit very similar dependence of both corrections on the tilting pattern.

We used BOSS to fit both $\Delta_{\mathrm{HF}}$ and $\Delta_{\mathrm{SOC}}$ within the 3D phase space. We also used BOSS to construct the surrogate model of PBEsol-calculated band gaps. We thus can use Eq. (1) to estimate how band gap depends on the tilting angles for both benchmark systems. **Figure S4** displays generally similar trends as in Figure 6 in the main text. It displays noticeable noise accompanied with the contours which is naturally due to the very few $\Delta_{\mathrm{HF}}$ and $\Delta_{\mathrm{SOC}}$ data points that are fit to the surrogate model. The chaos are especially pronounced with the more disordered $CsPbBr_3$ , indicating the deficiency in data points for a converged surrogate model. Nevertheless, as the trend of band-gap increase with tilting angles and the temperature-dependence of the average band gap are qualitatively reproduced, the approach represented in this section would be of interest to reduce the computation cost for a large number of hybrid-functional calculations.

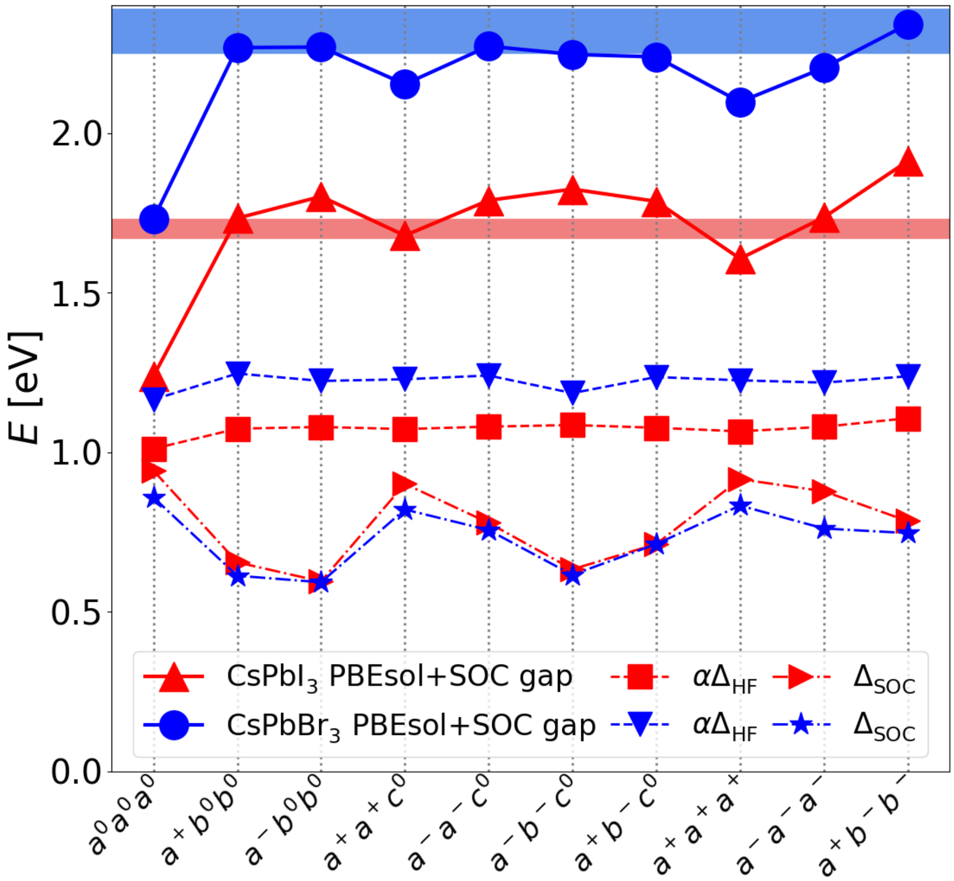


Figure S3: DFT band gap calculations for $CsPbI_3$ (red) and $CsPbBr_3$ (blue) for a series of tilting patterns. Shown are the PBEsol0+SOC band gap (solid lines), the correction due to the inclusion of HF exchange $\alpha\Delta_{\mathrm{HF}}$ (dashed lines), and the SOC correction $\Delta_{\mathrm{SOC}}$ (dot-dash lines). The light-red and light-blue shades indicate the experimentally measured band-gap ranged of $CsPbI_3$ and $CsPbBr_3$ , respectively.

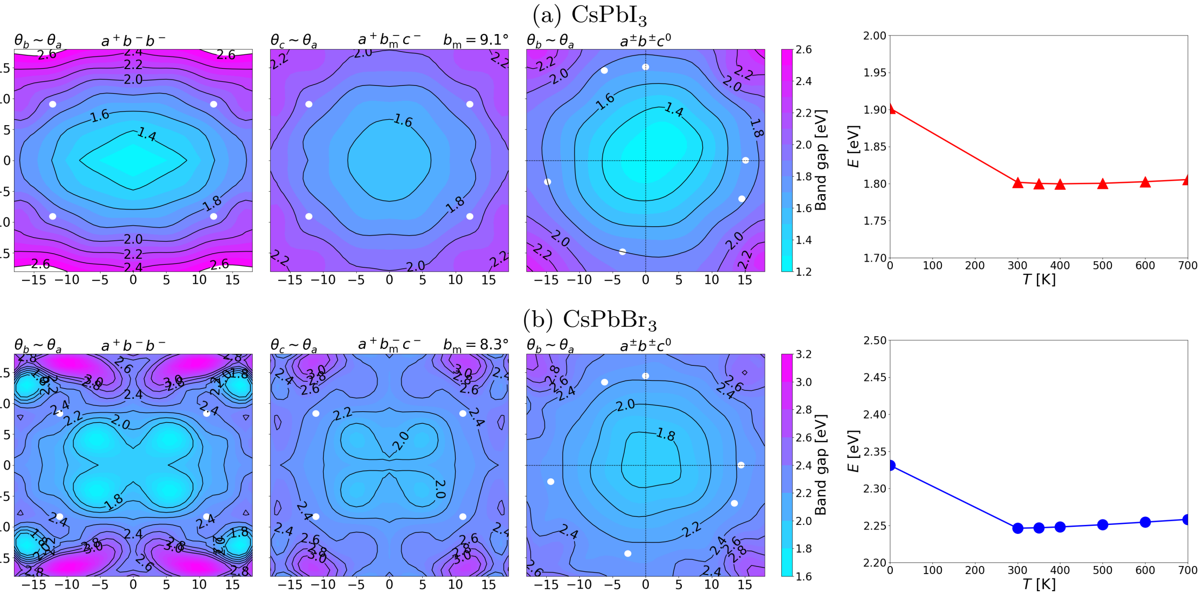


Figure S4: Band gaps of (a) $CsPbI_3$ and (b) $CsPbBr_3$ calculated based on a small number of $\Delta_{\mathrm{HF}}$ and $\Delta_{\mathrm{SOC}}$ data (shown are 2D cross-sections $a^+b^-b^-$, $a^+b^-_{\mathrm{m}}c^-$, and $a^{\pm}b^{\pm}c^0$)., as well as the thermally-weighted mean of band gaps as a function of temperature $T$.

# References

[1] J. Klarbring, *Phys. Rev. B* **2019**, *949* 104105.

[2] J. Even, L. Pedesseau, J.-M. Jancu, C. Katan, *J. Phys. Chem. Lett.* **2013**, *4* 2999.

[3] F. Brivio, K. T. Butler, A. Walsh, M. van Schilfgaarde, *Phys. Rev. B* **2014**, *89* 155204.

[4] A. Seidu, M. Dvorak, P. Rinke, J. Li, *J. Chem. Phys.* **2021**, *154* 074712.
